# Supplementary material for: Optimally Training a Cascade Classifier
Source: arXiv:1008.3742 source file (2010-08-23)
Supplement: Supplementary file 1 [file appendix.tex]

% LaTeX Source
% Author(s):     Chunhua Shen {chhshen@gmail.com}
% Creation:      Monday 03/05/2010 16:39.
% Last Revision: Monday 03/05/2010 16:59.

\appendices

\section{The Non-negativeness Constraint in Formulating \eqref{EQ:QP1} }

    If we enforce the non-negativeness constraint $ \bmu_1 - \bmu_2 \geq 0 $
    explicitly, then the primal problem becomes 
\begin{align}
            \min_{\w,\brho}
             ~& 
            \tfrac{1}{2} \brho ^\T \Q \brho - \theta \e^\T
            \brho,
          \notag\\  
            \quad {\rm s.t.} ~&\w \psd {\bf 0},
             {\bf 1}^\T \w = 1,
      \notag \\
      &
     {\rho}_i = ( \A \w )_i,
        i = 1,\cdots, m.
     \notag \\
     &
             \bmu_1 - \bmu_2 = \e^\T \brho \geq 0.
            \label{EQ:QP1B}
\end{align}

% EoF
